# Supplementary material for: Self-explaining deep models with logic rule reasoning
Source: arXiv:2210.07024 source file (2022-10-18)
Supplement: Supplementary file 1 [file appendix4_codes.tex]

\section{Codes}
Please read README file before you run the code.

\textbf{atom\_pool.py}
This file contains implementation related to the atom.

\textbf{dataset.py}
This file contains implementation of data loading and dataset objects for training.

\textbf{model.py}
This file contains implementation of the models.

\textbf{train\_eval.py}
This file contains the implementation of training, validation, and testing of the models.

\textbf{utils.py}
This file contains the implementation of argument parsing, and seed reset.

\textbf{base.py}
This file trains the base backbone network. Results are saved in "\emph{./result}" directory. The default base model is set to BERT and default dataset is set to Yelp.

\textbf{update\_latest\_base\_model.py}
This file creates "\emph{./save\_dir/base\_model}" directory and copies the latest trained base model into the directory.
    
\textbf{extract\_train\_embedding.py}
This file extracts embeddings of the training dataset from the base model.
    
\textbf{build\_atom\_pool.py}
This file builds a pool of atoms from train dataset. For textual datasets, control the number of atoms by the "\emph{--num\_atoms}" argument (default: 5000).

\textbf{sample\_rules\_for\_pretrain.py}
This file searches for sample rule candidates to pretrain the consequent estimator. Control the generality of rules by the "\emph{--min\_df}" argument (default: 200).
    
\textbf{pretrain\_consequent\_estimator.py}
This file pretrains the consequent estimator. Control the number of rules for pretraining by the "\emph{--pretrain\_samples}" argument (default: 10000).

\textbf{rule\_gen.py}
This file trains the main model, antecedent generator. You can control the number of atoms in a rule by the "\emph{--max\_rule\_len}" argument (default: 4). The results are saved in "\emph{./result}" directory.

\textbf{extract\_explanation.py}
This file extracts explanations from the latest trained model. The explanations are saved in the same directory as the model.
